# Supplementary material for: Fair Allocation of Indivisible Goods: Improvement and Generalization
Source: arXiv:1704.00222 source file (2017-07-23)
Supplement: Supplementary file 1 [file appendix.tex]

Here comes the appendix.
